# Supplementary material for: Coherence of dipole-forbidden Rydberg excitons in Cu$_2$O measured by polarization- and time-resolved multi-photon spectroscopy
Source: arXiv:2507.22717 source file (2025-07-30)

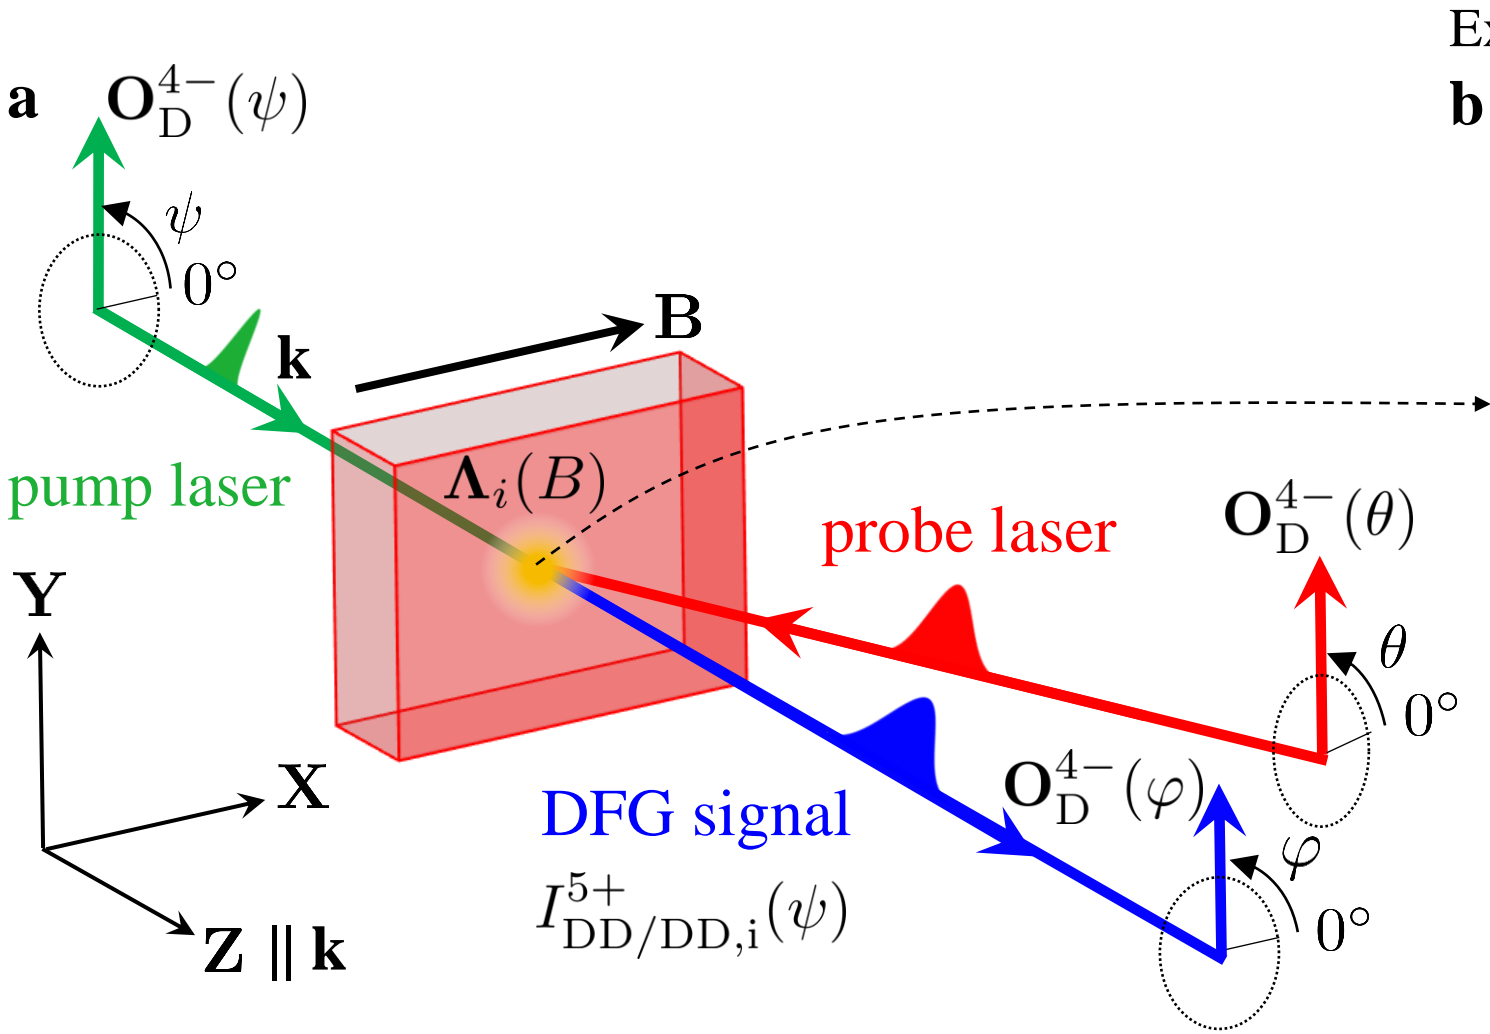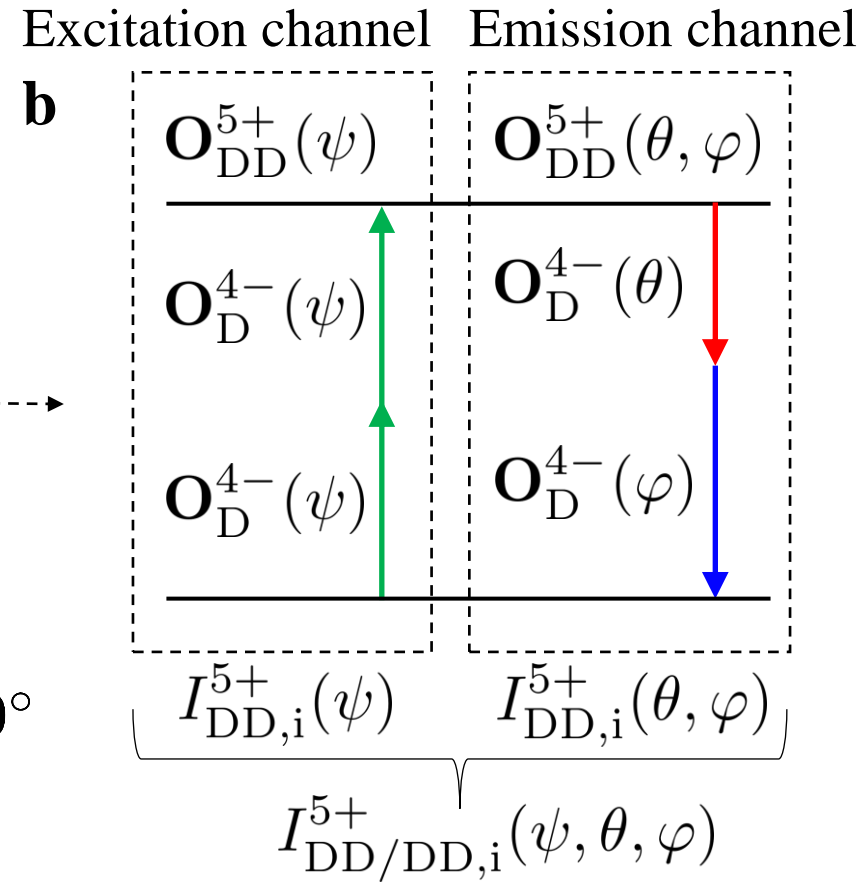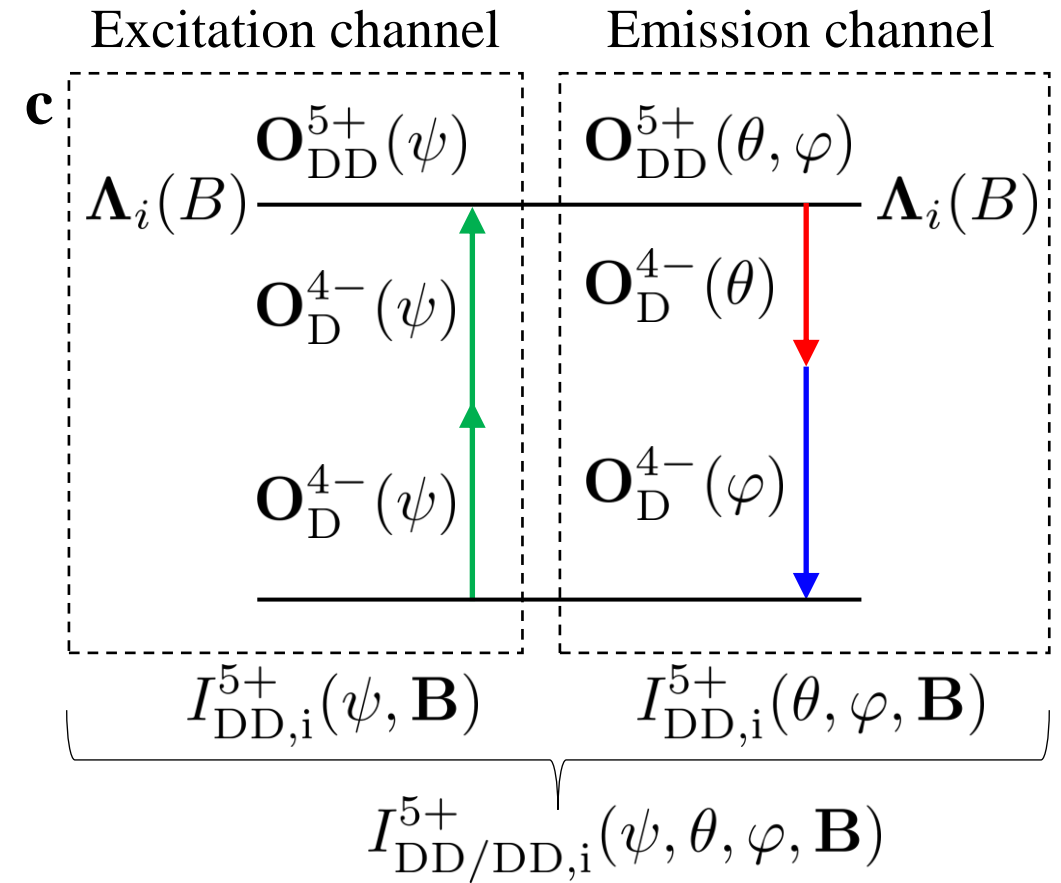

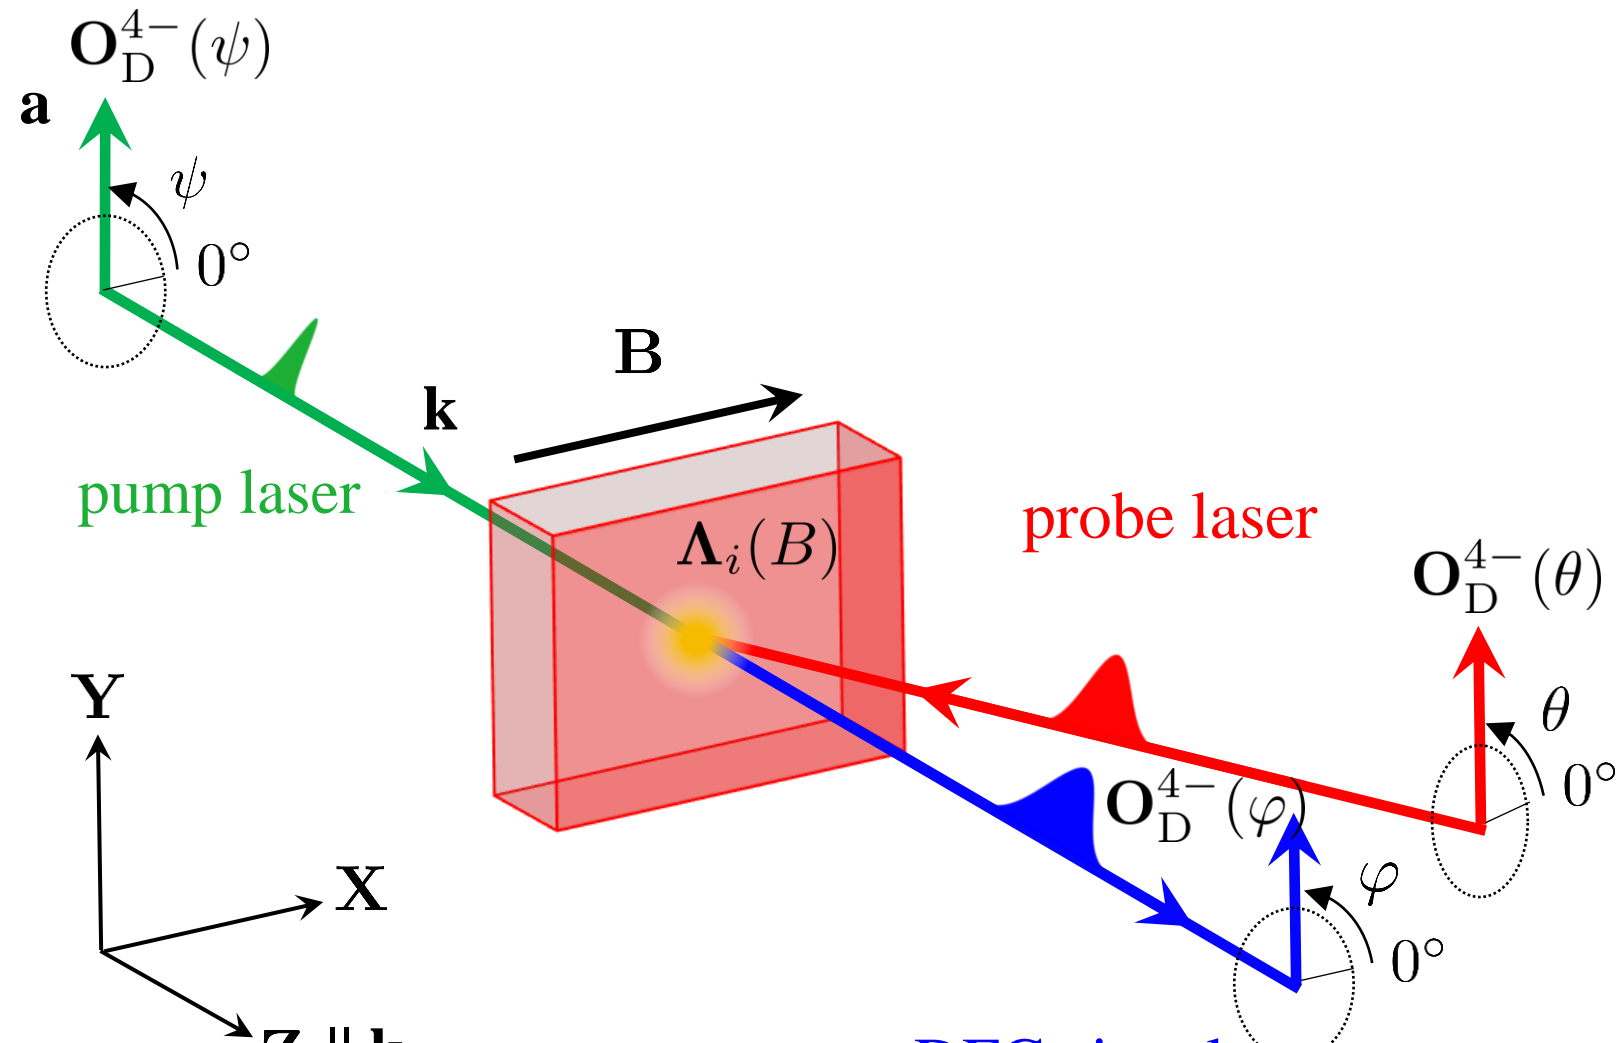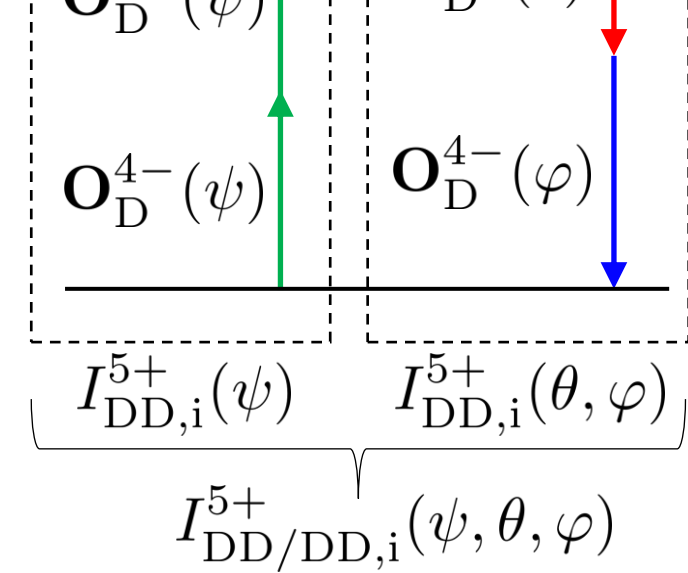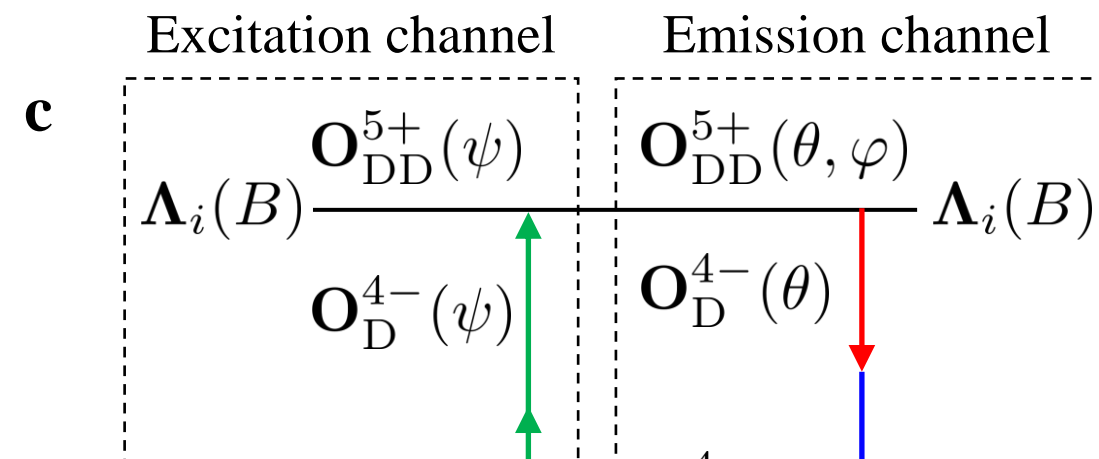

Supplement: Supplementary file 1 [file exp_geo_SI.pdf]
